# Supplementary material for: Measuring I2P Censorship at a Global Scale
Source: arXiv:1907.07120 source file (2019-07-16)
Supplement: Supplementary file 1 [file appendix.tex]

\section{Appendix}
\label{sec:appendix}

\begin{figure}[ht]
\centering
\includegraphics[width=\columnwidth,height=0.39\textwidth]{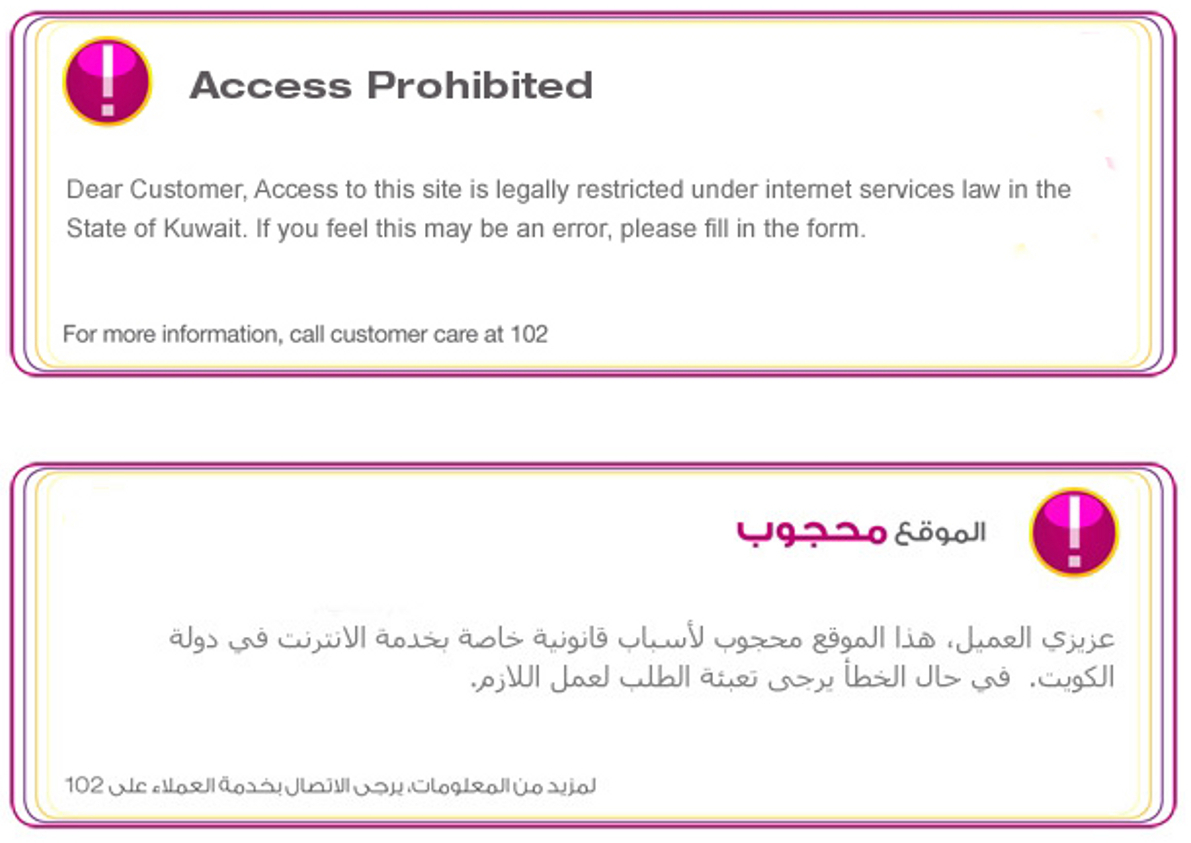}
\caption{Example block page from Kuwait.}
\label{fig:kuwait}
\end{figure}

\begin{figure}[ht]
\centering
\includegraphics[width=\columnwidth,height=0.33\textwidth]{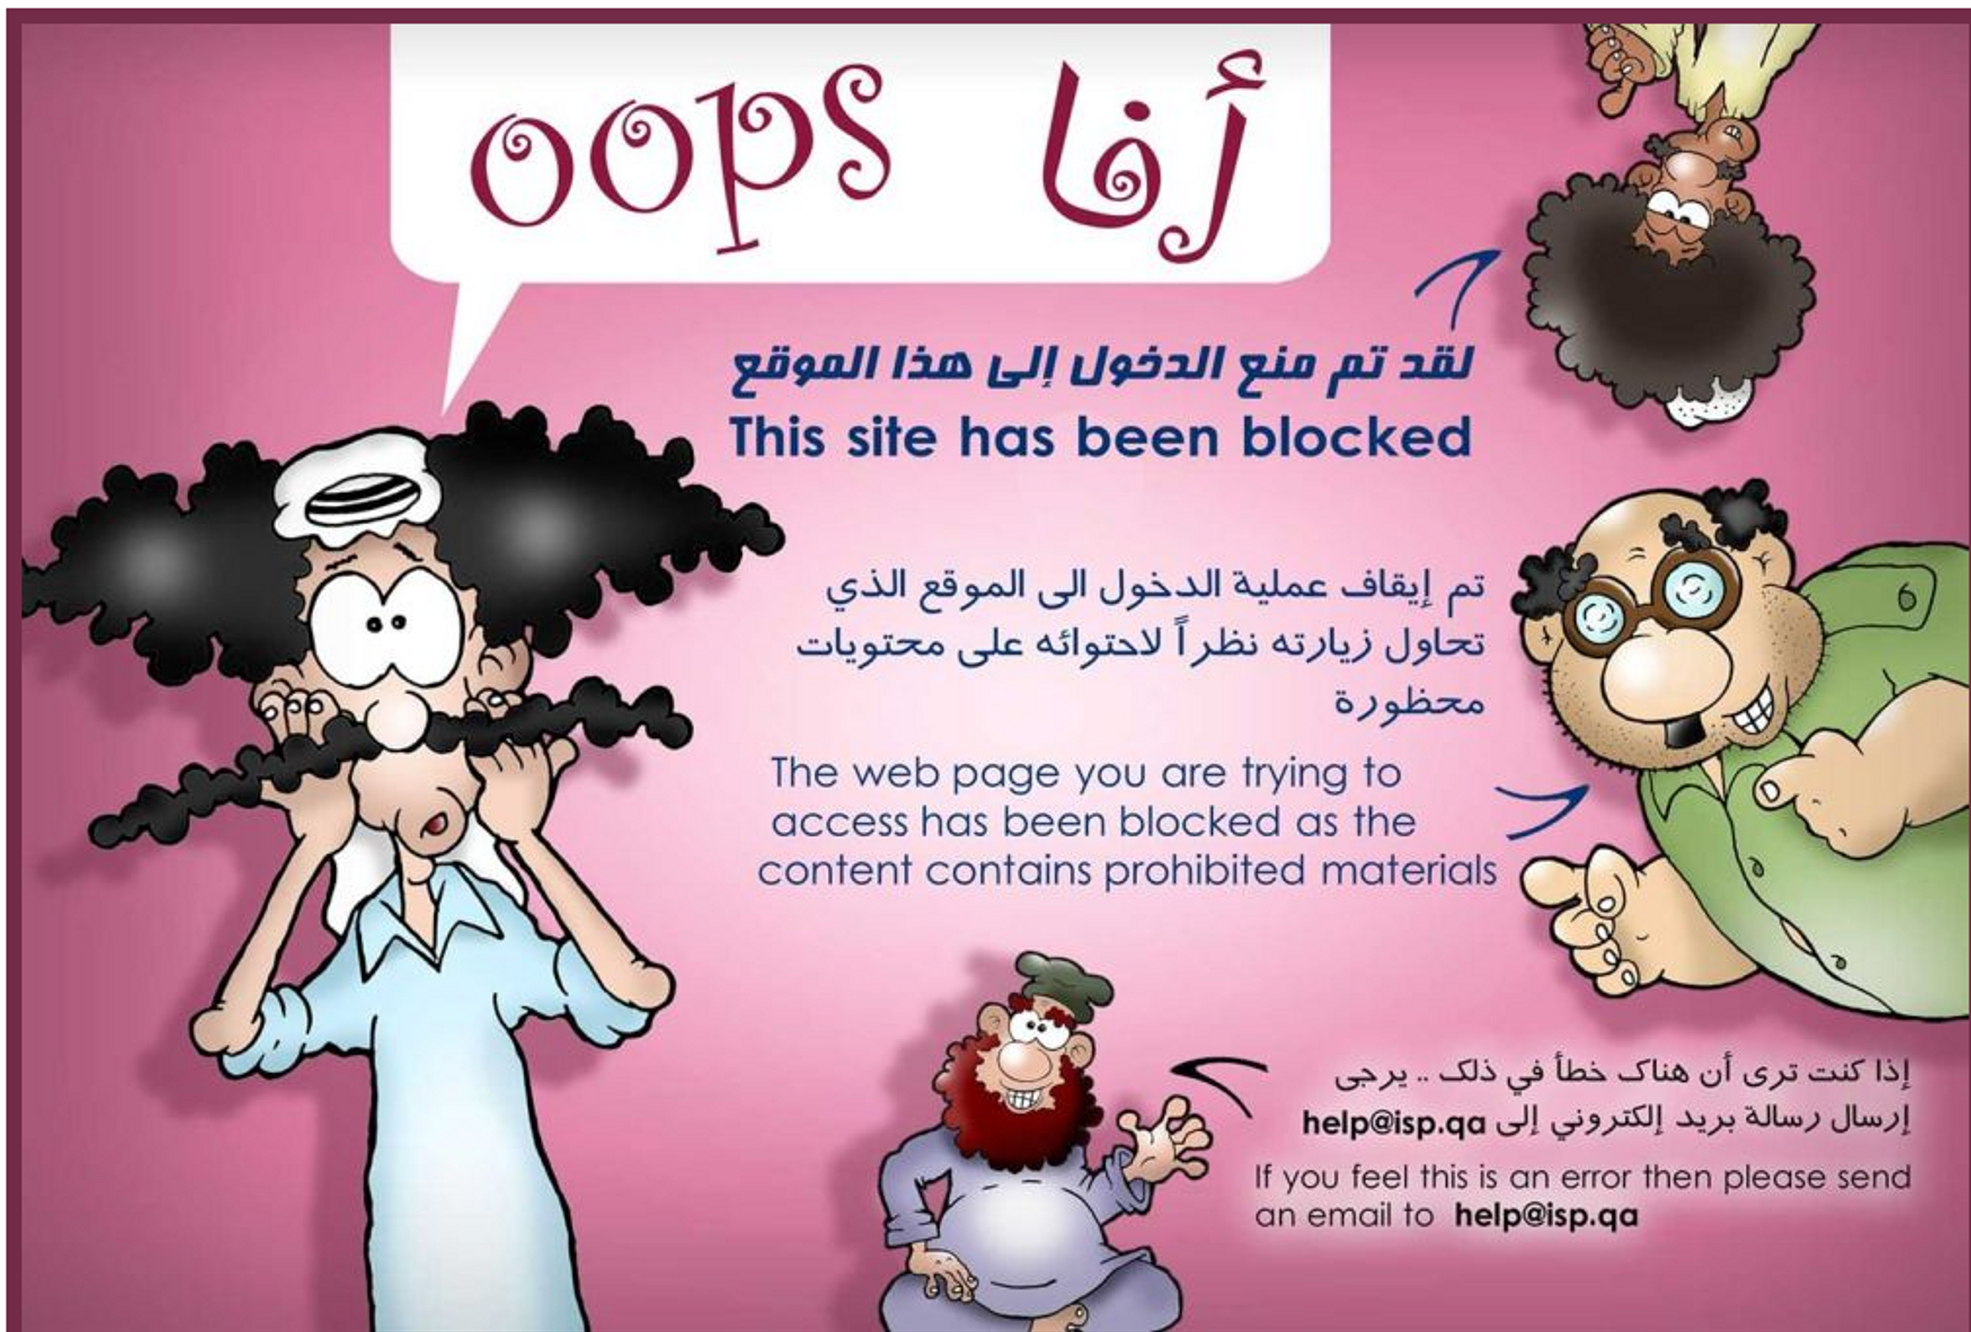}
\caption{Example block page from Qatar.}
\label{fig:qatar}
\end{figure}

\begin{figure*}[t]
\centering
\includegraphics[width=0.8\textwidth]{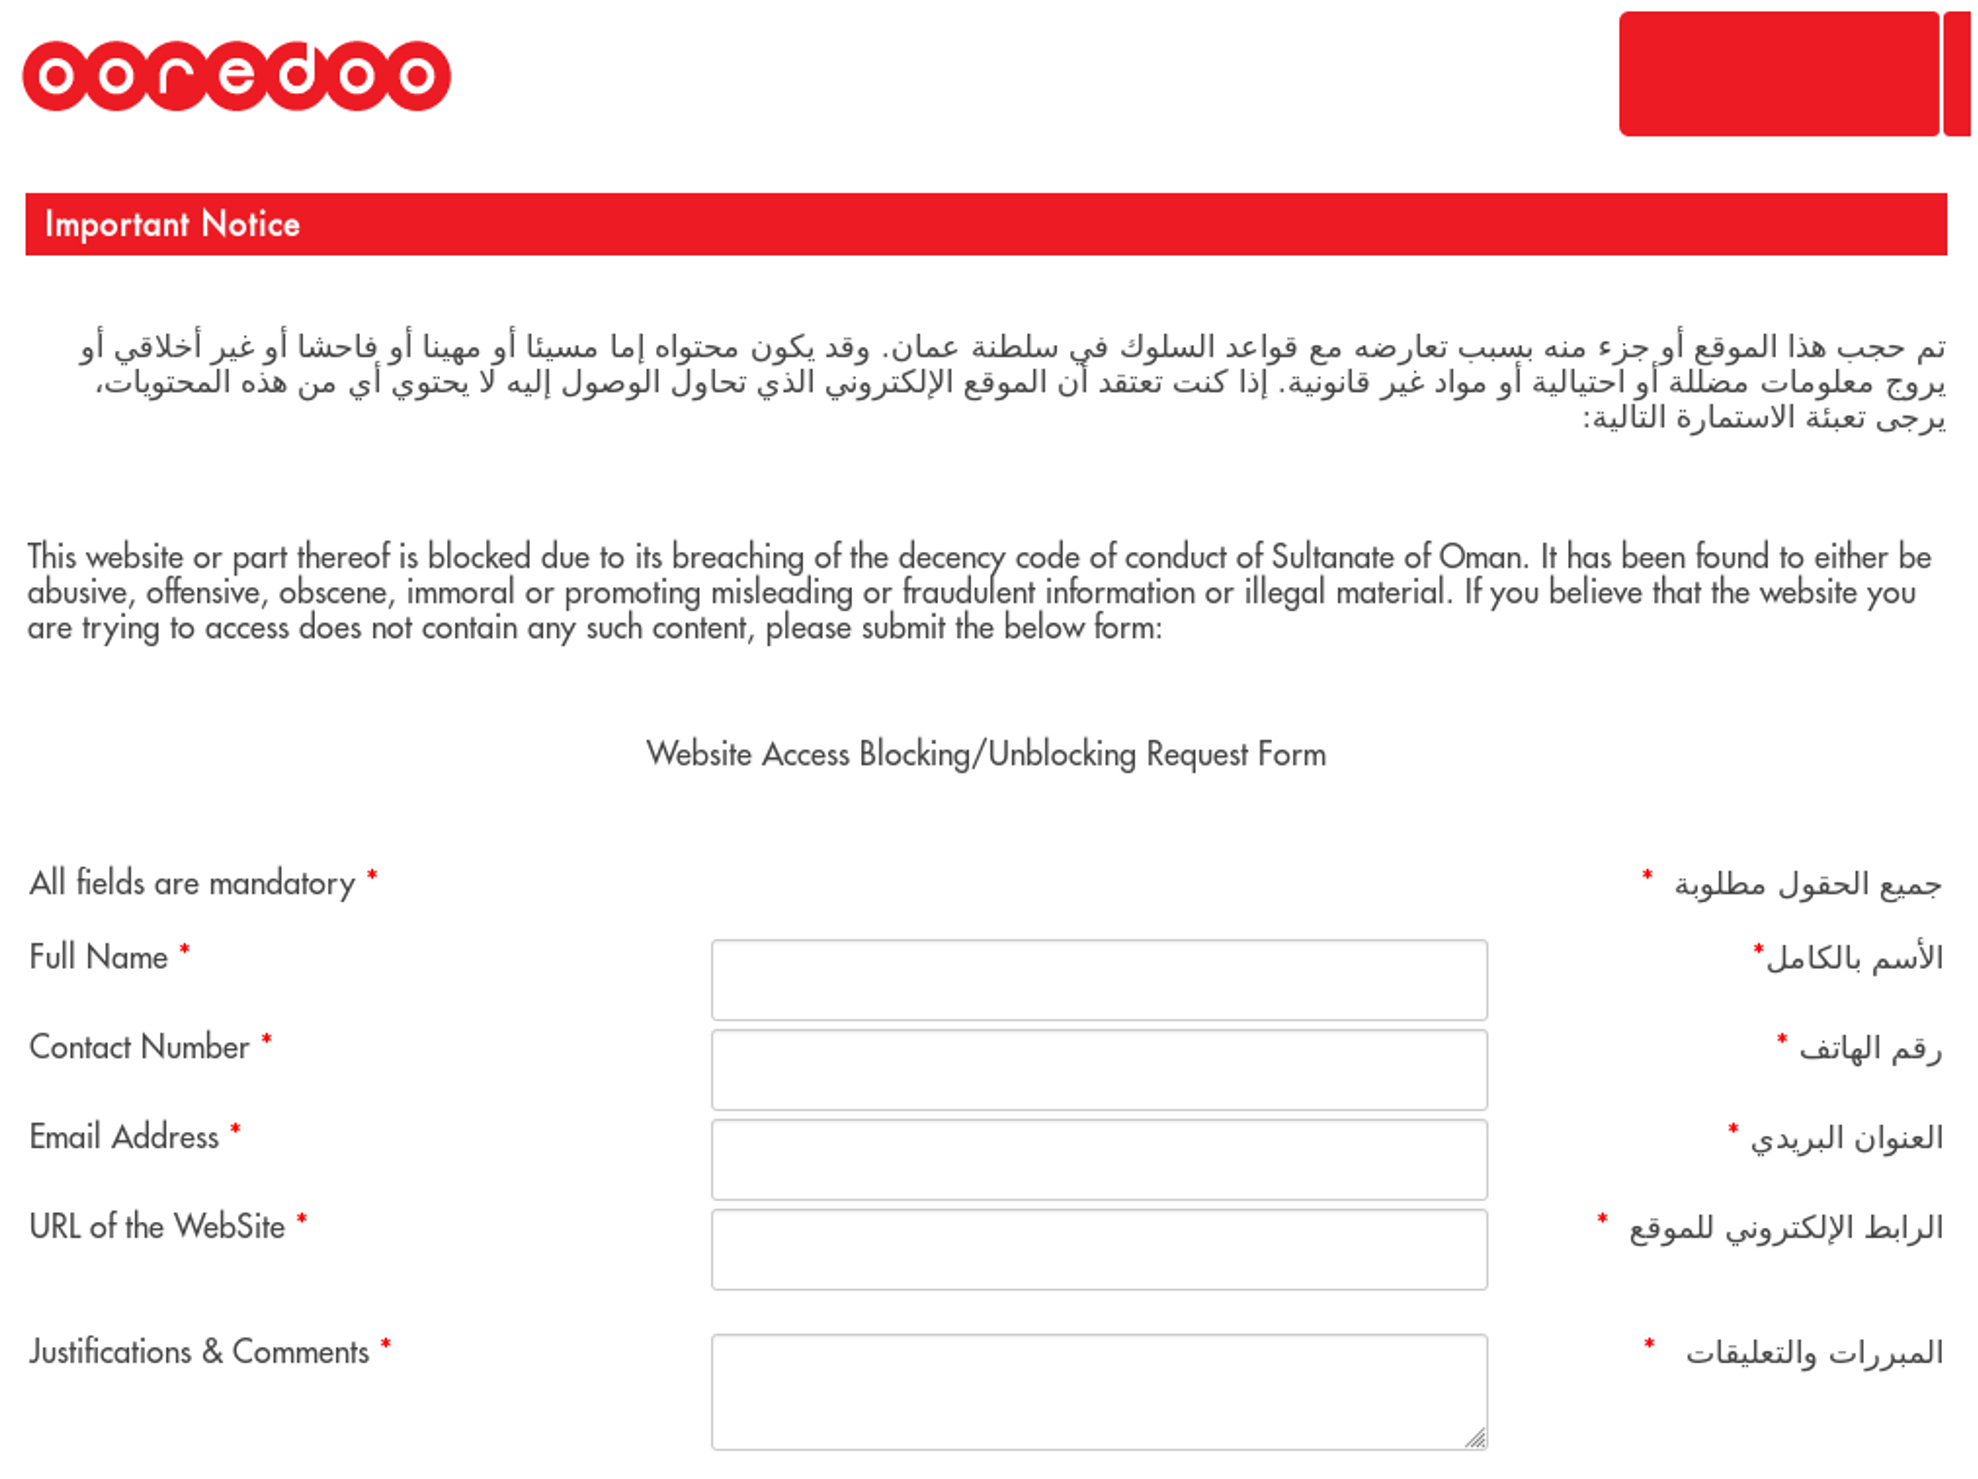}
\caption{Example block page from Oman.}
\label{fig:oman}
\end{figure*}

\begin{table*}[t]
\centering
\begin{tabular}{|c|c|c|c|c|}
\hline
\multirow{2}{*}{Country} & \multicolumn{2}{c|}{Domain-name-based blocking}                                                                        & \multirow{2}{*}{TCP packet injection}                               & \multirow{2}{*}{Block page} \\ \cline{2-3}
                         & DNS                                                                                                       & SNI        &                                                                     &                             \\ \hline
China                    & \begin{tabular}[c]{@{}c@{}}geti2p.net\\ reseed.i2p-projekt.de\\ netdb.i2p2.no\\ i2p.mooo.com\end{tabular} & N/A        & N/A                                                                 & N/A                         \\ \hline
Iran                     & N/A                                                                                                       & N/A        & i2p-projekt.de                                                      & N/A                         \\ \hline
Oman                     & N/A                                                                                                       & geti2p.net & \begin{tabular}[c]{@{}c@{}}geti2p.net\\ i2p-projekt.de\end{tabular} & i2p-projekt.de              \\ \hline
Qatar                    & N/A                                                                                                       & geti2p.net & \begin{tabular}[c]{@{}c@{}}geti2p.net\\ i2p-projekt.de\end{tabular} & i2p-projekt.de              \\ \hline
Kuwait                   & N/A                                                                                                       & N/A        & i2p-projekt.de                                                      & i2p-projekt.de              \\ \hline
\end{tabular}
\caption{Summary of censored countries, filtered I2P services, and blocking techniques detected.}
\label{tab:sum_block}
\end{table*}
